# Supplementary material for: iDet3D: Towards Efficient Interactive Object Detection for LiDAR Point Clouds
Source: arXiv:2312.15449 source file (2023-12-24)
Supplement: Supplementary file 1 [file 1_details.tex]

\section{Detailed iDet3D Architecture}

iDet3D is built upon the backbone of IA-SSD~\cite{zhang2022not} with additional components for interactive functionality.
In this section, we provide the detailed architecture of iDet3D.
The point encoder of iDet3D can be represented with respect to the sequential set abstraction (SA) blocks, \emph{i.e.,}
{\small
\begin{equation*}
\begin{aligned}
\text{- KITTI: } &P(16384, 4+3) \rightarrow \text{SA} \rightarrow P(4096, 64+3) \\
&\rightarrow \text{SA} \rightarrow P(1024, 128+3) \rightarrow \text{SA} \\
&\rightarrow P(512, 256+3) \rightarrow \text{SA} \rightarrow P(256, 64+3)  \\
&\rightarrow \text{NCS} \rightarrow P(256, 512+4) \rightarrow \text{CA} \\
&\rightarrow P(256, 512+4) \rightarrow \text{SCP} \rightarrow P(256, 512+4+4). \\
\end{aligned}
\end{equation*}

\vspace{-0.5\baselineskip}
\begin{equation*}
\begin{aligned}
\text{- nu}&\text{Scenes: } P(65536, 5+10) \rightarrow \text{SA} \rightarrow P(16384,64+10) \\
&\rightarrow \text{SA} \rightarrow P(4096, 128+10) \rightarrow \text{SA} \\
&\rightarrow P(2048, 256+10) \rightarrow \text{SA} \rightarrow P(1024, 64+10) \\ 
&\rightarrow \text{NCS} \rightarrow P(1024, 512+11) \rightarrow \text{CA} \\
&\rightarrow P(1024, 512+11) \rightarrow \text{SCP} \rightarrow P(1024, 512+11+11). \\
\end{aligned}
\end{equation*}
}
In these representations, $P(N, D)$ denotes a set of $N$ point embeddings each of which is a $D$-dimensional vector,
NCS, CA, and SCP refer to our proposed negative click simulation, the centroid aggregation layer of our backbone~\cite{zhang2022not}, and spatial click propagation module, respectively.
As each intermediate layer of our encoder additionally takes $C$-dimensional \emph{class-wise} click encodings via concatenation (see the dense click guidance strategy in Section 3.3), we represent the concatenated dimension with the plus $(+)$ operation.
The same representation method is applied to the case of \emph{class-wise} correlation maps produced by the SCP module.
The NCS strategy adds one additional dimension to the class-wise click encodings and correlation maps with respect to negative clicks.

The following 3D detection heads, which are composed of four fully-connected layers, take the output point embeddings of the SCP module as its input.
