# Supplementary material for: iDet3D: Towards Efficient Interactive Object Detection for LiDAR Point Clouds
Source: arXiv:2312.15449 source file (2023-12-24)
Supplement: Supplementary file 2 [file 2_vis_components.tex]

\section{Qualitative Analysis of Our Components}

In this study, we build a vanilla version of interactive 3D object detector and overcome its limitations by proposing
the negative click simulation (NCS) strategy and two click propagation approaches, dense click guidance (DCG) and spatial click propagation (SCP).
This section aims to show the effectiveness of each component by providing qualitative visualizations of 3D object detection results.

%propose a negative click simulation (NCS) strategy for 3D interactive object detection and two click propagation approaches, dense click guidance (DCG) and spatial click propagation (SCP).
%We visualize several examples to show the effectiveness of each component.

\subsection{Negative Click Simulation}

As mentioned in Section 3.2, we propose a negative click simulation (NCS) strategy to sample \emph{challenging background points that are likely to be mistakenly predicted to foregrounds (false positives)} as negative clicks during training.
We provide visual samples of negative clicks from our NCS in Fig.~\ref{supplefig:ncs}.
% With consideration of the purpose of our NCS, it is intuitive that negative clicks are not incorporated into the network, the negative points sampled by the NCS located inside the false-positive predictions.
% For better visualization, we visualize various predictions including low-confidence predictions (with a confidence threshold of 0.1).  
As shown in the figure, the sampled negative clicks lie inside the false-positive predictions, and iDet3D fails to filter out these cases without negative click encoding into the network.
In other words, the NCS successfully localizes confusing background regions as negative clicks during training only with the positive ground truth boxes.

\begin{figure*}[t] %%% t: top, b: bottom, h: here
\centering
\includegraphics[width=1.0\textwidth]{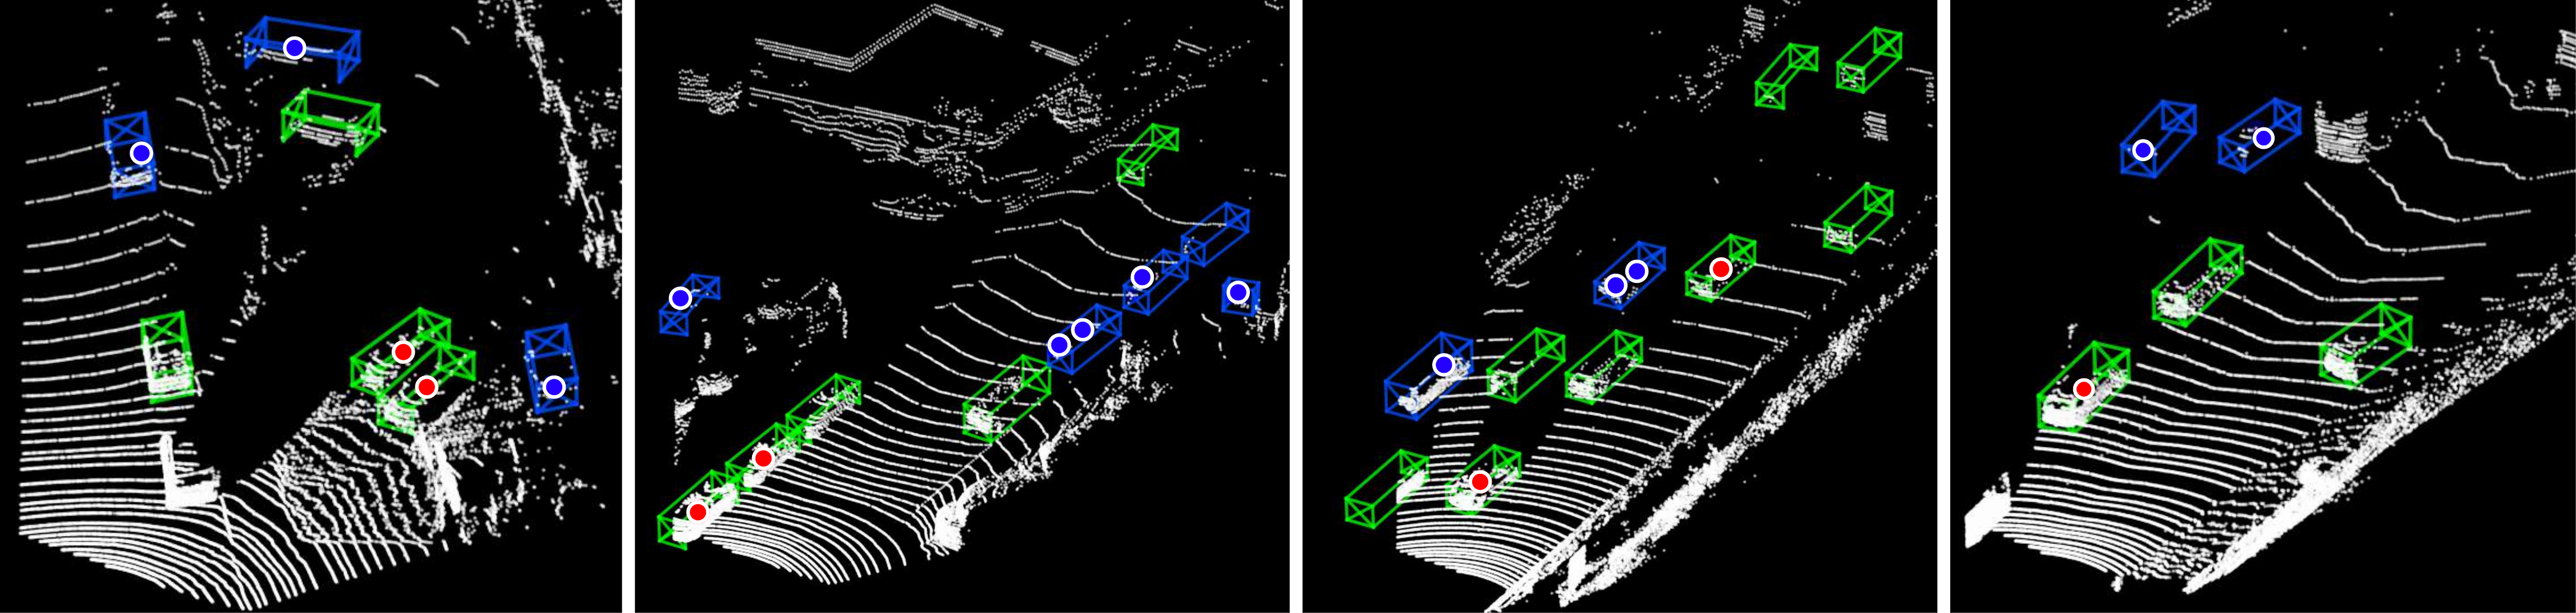}
\caption{
    Visualization of the negative clicks (\textcolor{blue}{blue circle}) sampled by our negative click simulation (NCS).
    Note that these clicks are simulated during training only with the ground truth corresponding to the true positives (\textcolor{green}{green}).
    The NCS successfully samples the points in false positive (\textcolor{blue}{blue box}) predictions.
    For visualization, we do not encode the negative clicks into the network but only sample them.
}

\label{supplefig:ncs}
\end{figure*}

\subsection{Dense Click Guidance}
To take full advantage of user-guided information throughout the point encoder, we propose dense click guidance (DCG) approach in Section 3.3, which feeds click encodings into not only the input point scenes but also the intermediate feature embeddings.
We expect that iDet3D can sustain user intention without dropping crucial points for precise prediction by adopting this method.
One of the straightforward ways to figure out how DCG works for iDet3D is to deep dive into the downsampled points of the encoder.
Therefore, We visualize which points are preserved after subsequent downsampling layers at the output of the encoder
As illustrated in Fig~\ref{supplefig:dcg}, iDet3D with DCG can detect user-specified objects with explicit interaction while maintaining neighboring points of user clicks, unlike the vanilla model.

\subsection{Spatial Click Propagation}
For a better understanding of our spatial click propagation (SCP) module, we visualize several samples of correlation maps produced by SCP.

\paragraph{Correlation map of negative clicks.}
As described in Section 3.3, negative clicks in our system can suppress not only the specified background points but also high-related other points.
\emph{i.e.,} a single negative click can eliminate more than one false-positive prediction. 
To further validate the effectiveness of the SCP on negative clicks, we visualize the correlation maps from the SCP on negative interactions.
As depicted in Fig~\ref{supplefig:scp_neg}, the correlation maps from negative clicks highlight background points while showing low intensities for points inside the ground truth boxes.

\paragraph{Correlation map of positive clicks.}
We visualize more samples of the SCP correlation maps from positive clicks on foreground objects in Fig.~\ref{supplefig:scp_pos}.
The SCP of our iDet3D successfully highlights other points belonging to the same class of the class-specific encoding. 

\begin{figure*}[t] %%% t: top, b: bottom, h: here
\centering
\includegraphics[width=1.0\textwidth]{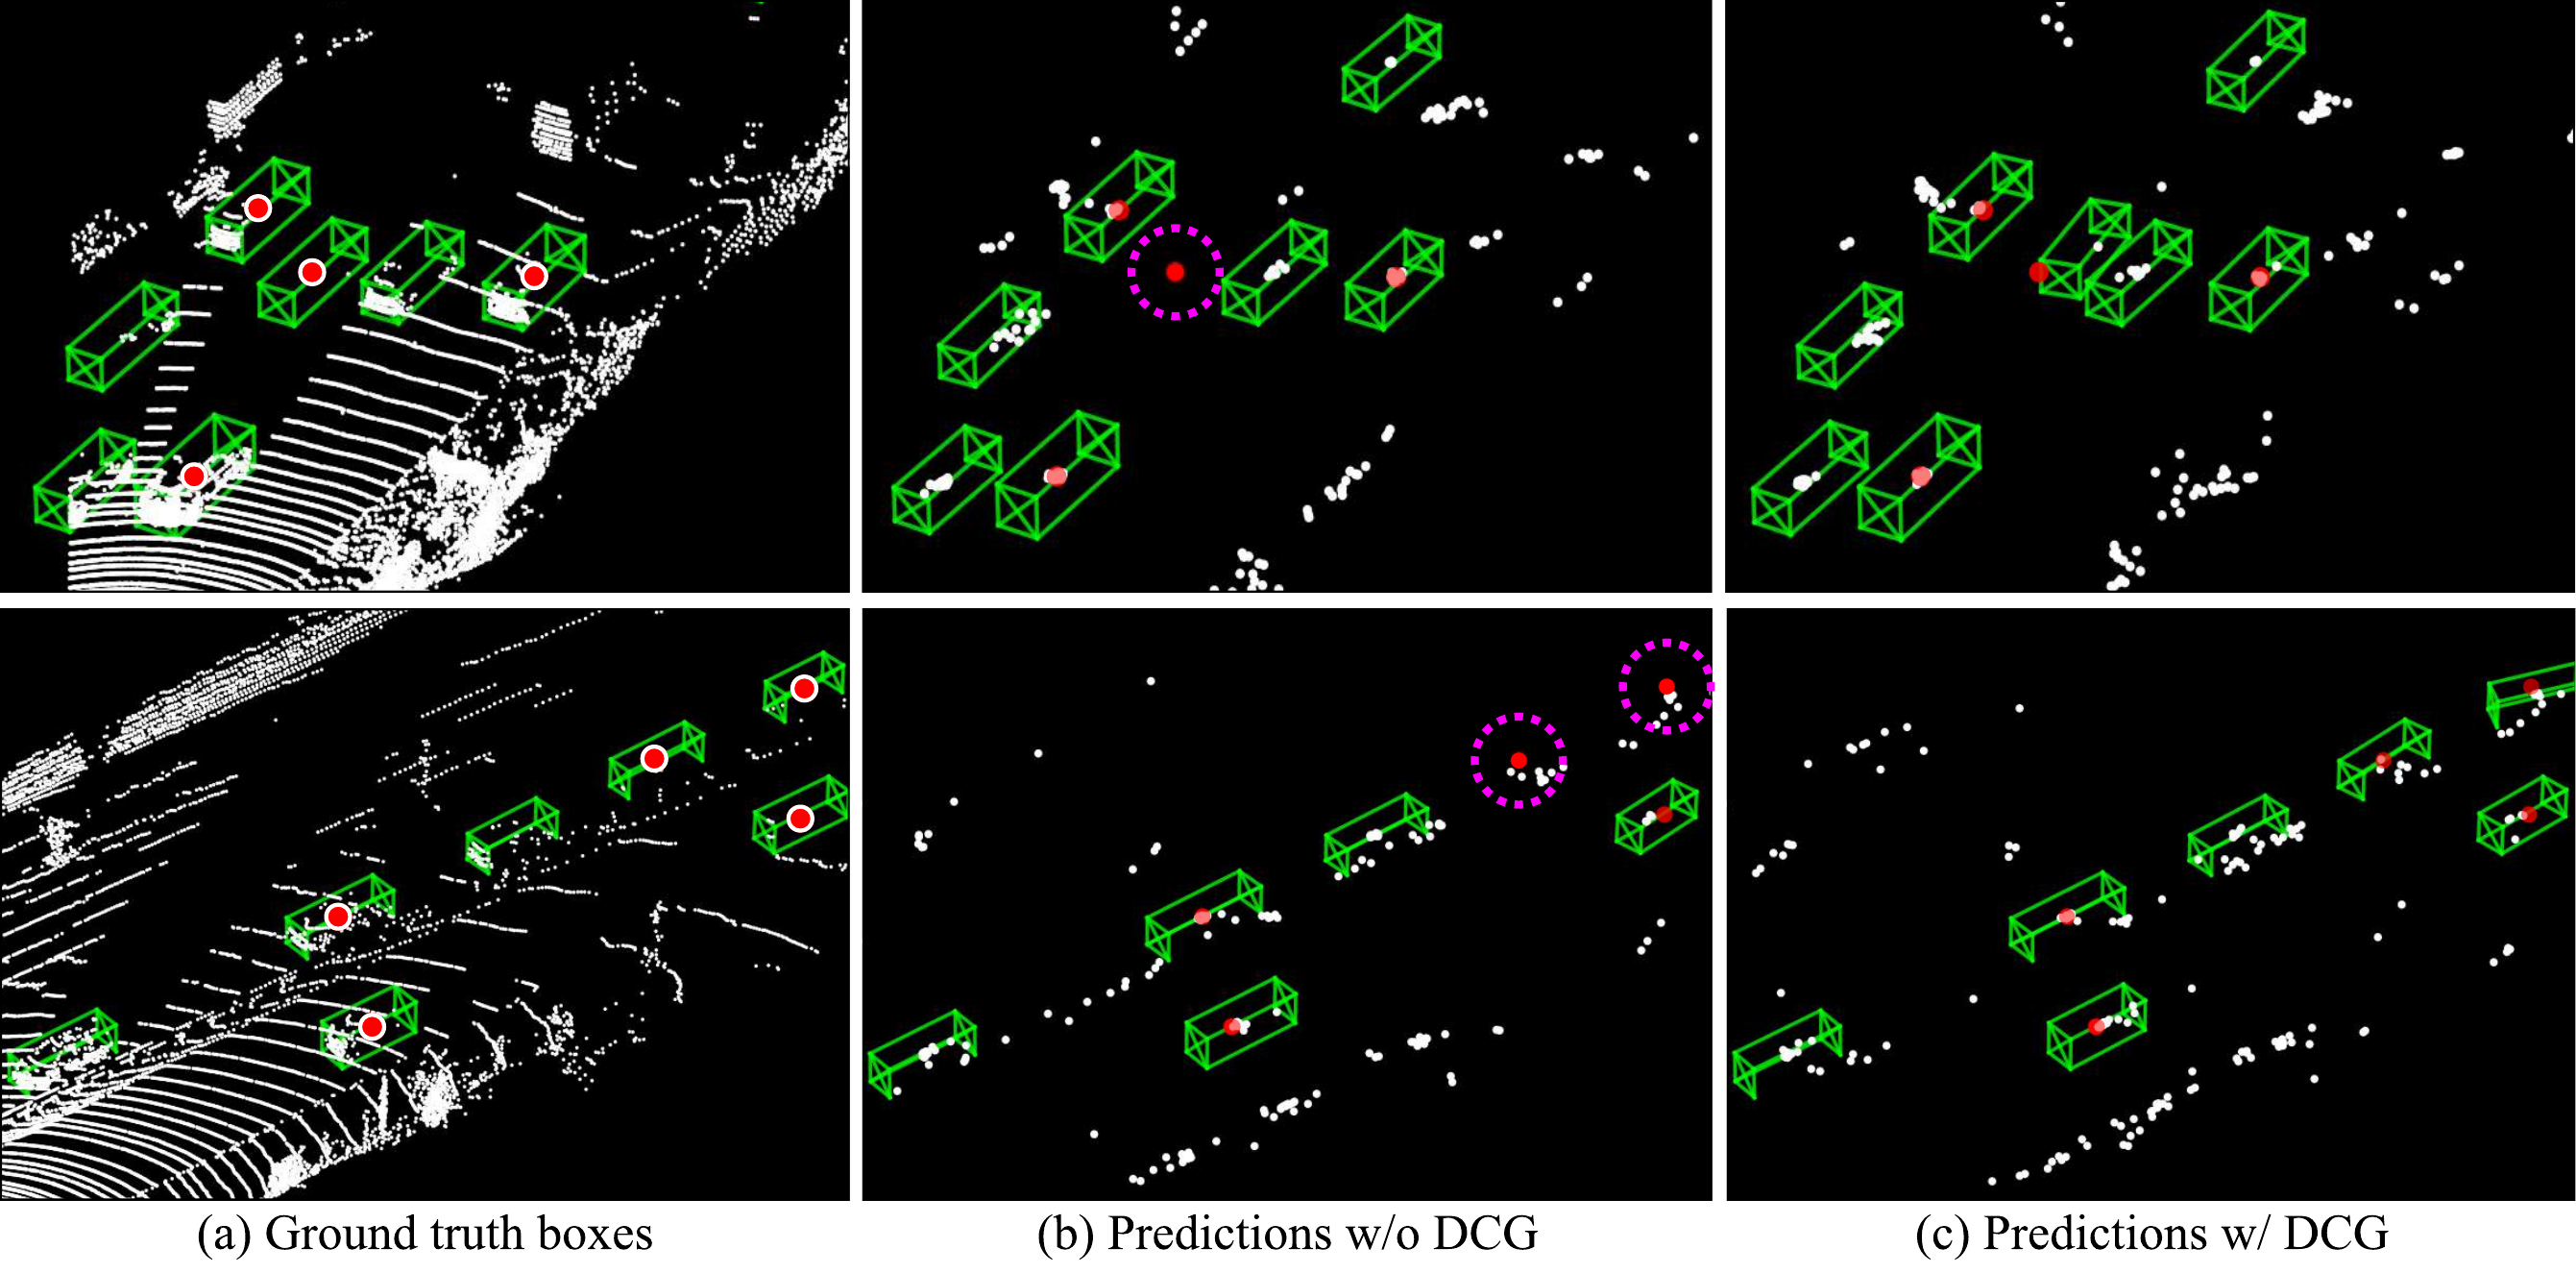}
\caption{
    Visualization of the downsampled points and prediction results from vanilla iDet3D without dense click guidance (DCG) and iDet3D with DCG.
    (a) For a given scene and user clicks (\textcolor{red}{red}) on target car objects (\textcolor{green}{green}), (b) vanilla iDet3D without dense click guidance tends to generate false-negative predictions (\textcolor{brightpink}{pink} circle).
    It is noteworthy that foreground points inside the ground truth boxes corresponding to the false positives can be lost through downsampling even with explicit positive clicks.
    Meanwhile, (c) iDet3D with DCG can retain such foreground points after downsampling stages and successfully predict the corresponding bounding boxes.
}

\label{supplefig:dcg}
\end{figure*}

\begin{figure*}[t] %%% t: top, b: bottom, h: here
\centering
\includegraphics[width=1.0\textwidth]{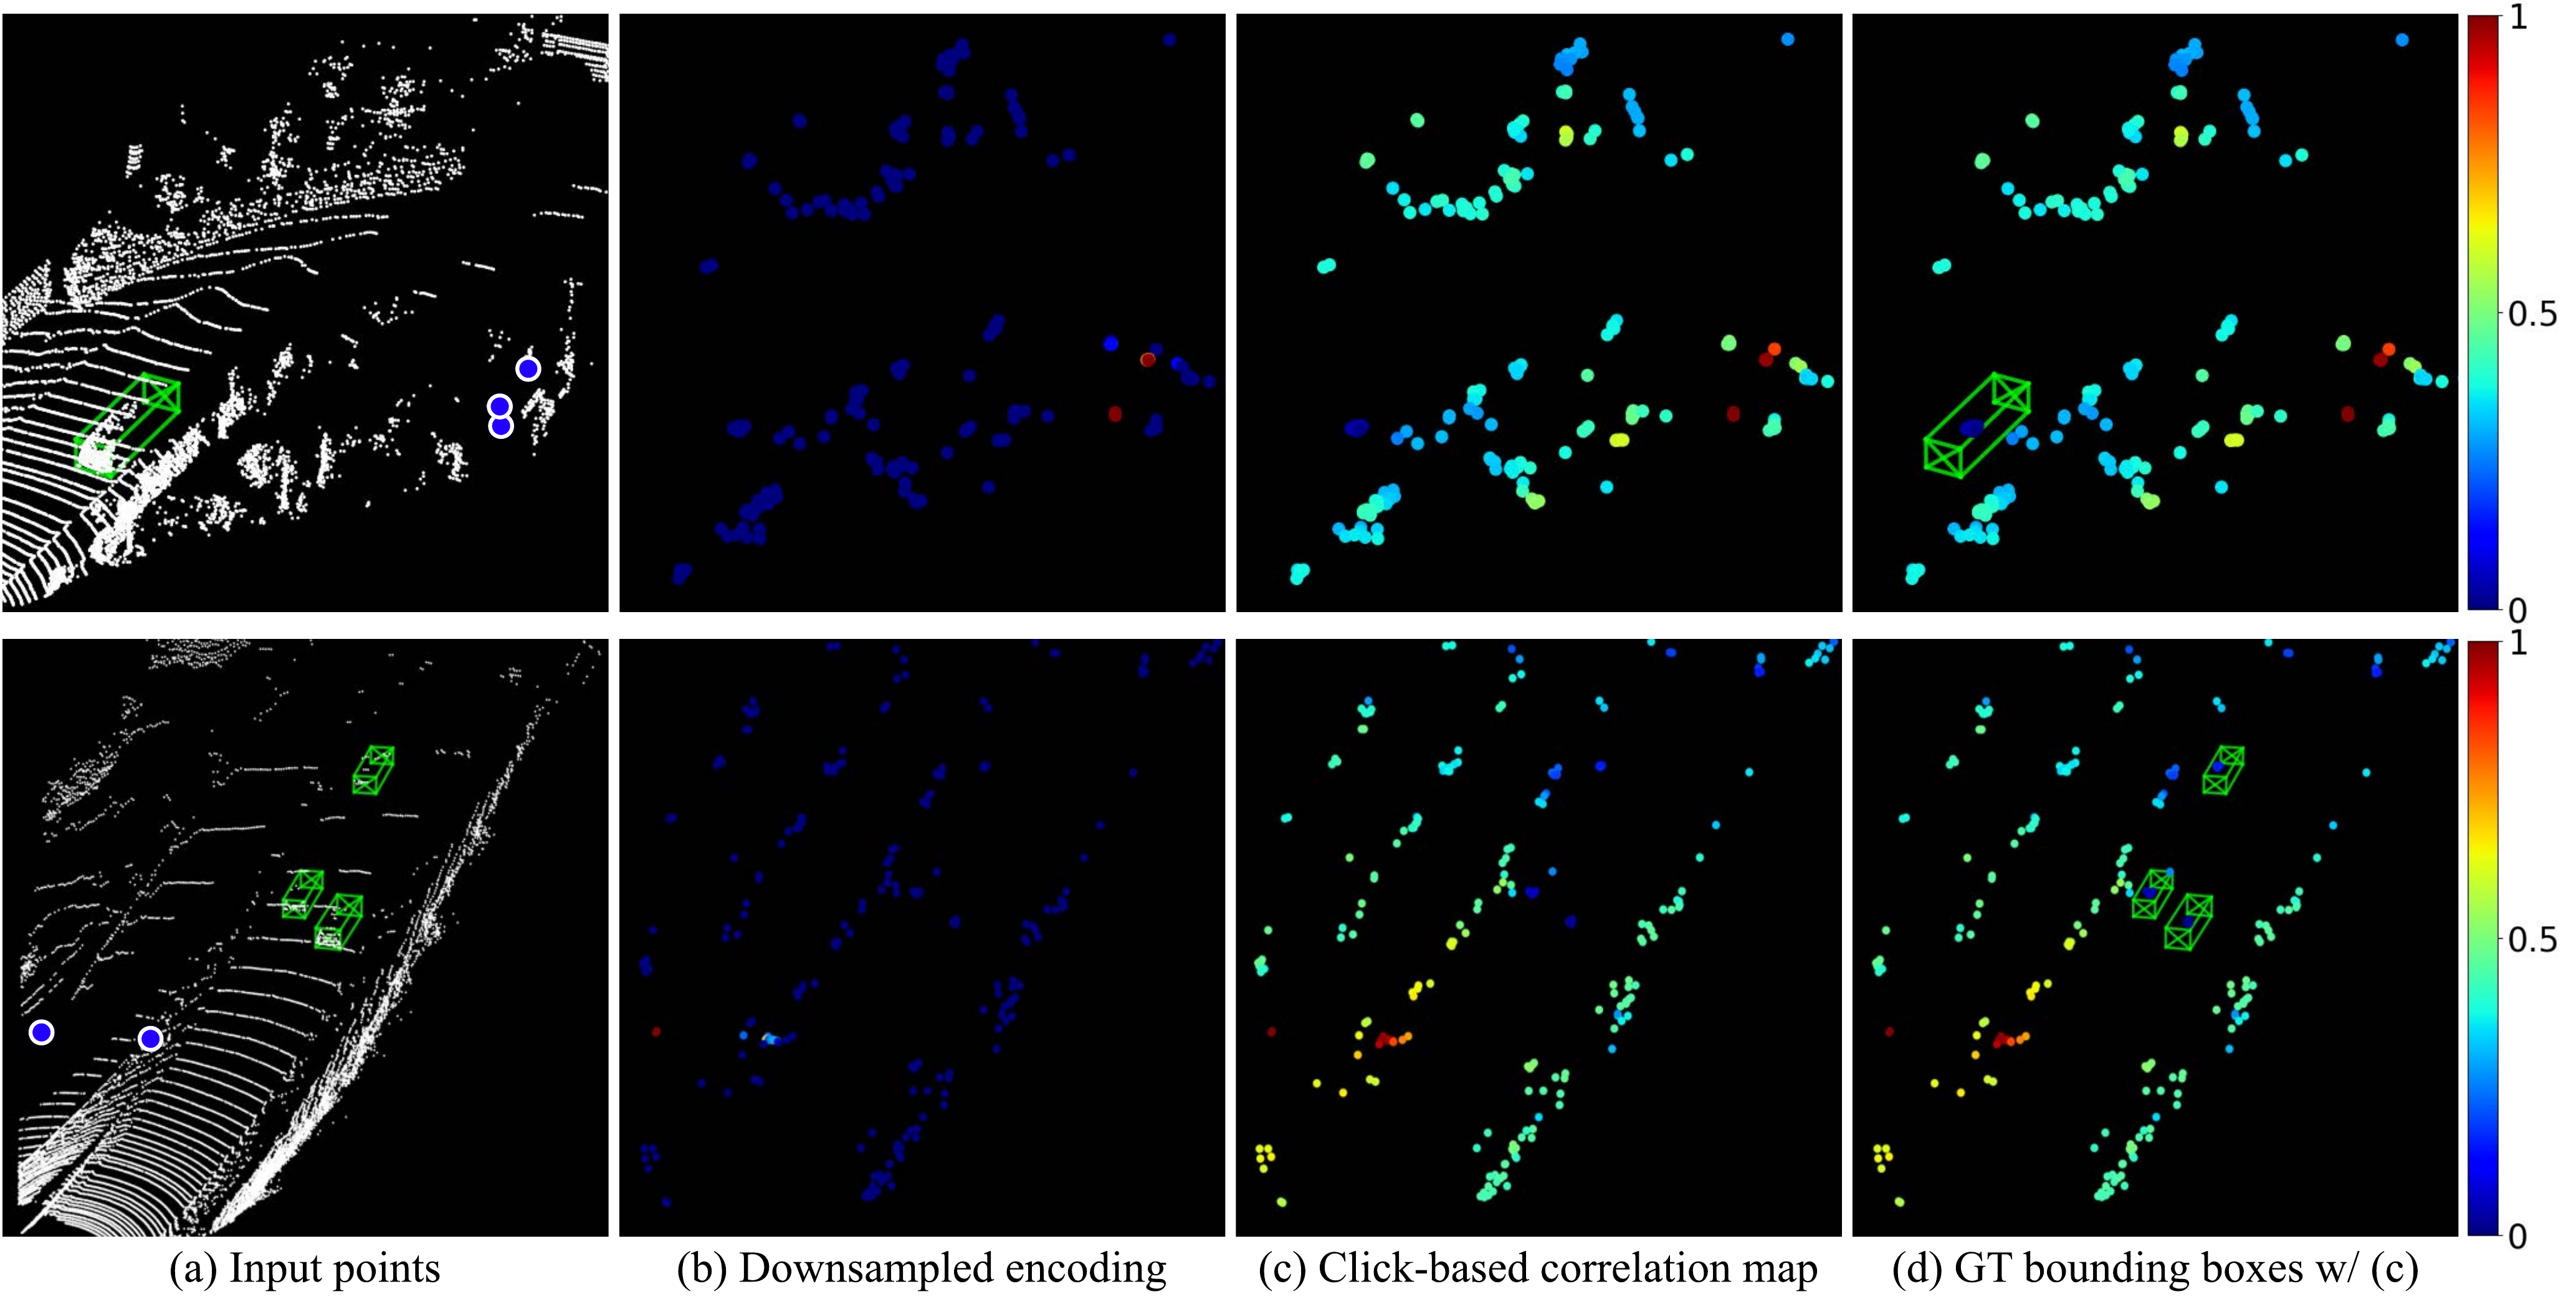}
\caption{
    An example of correlation map generation from negative clicks using spatial click propagation (SCP) module (visualized in the scale of [0,1]).
    (a) Input point scenes overlaid with ground truth boxes (\textcolor{green}{green}) and negative clicks (\textcolor{blue}{blue}).
    (b) A negative click encoding $U'$ for $N'$ downsampled points.
    (c) A correlation map $S$ generated by the SCP based on negative clicks and
    (d) visualization with the ground-truth 3D bounding boxes.
    Note that points of the foreground points inside the ground truth boxes have low similarity values with negative clicks while highlighting the background points (like roads or trees).
}
\label{supplefig:scp_neg}
\end{figure*}

\begin{figure*}[t] %%% t: top, b: bottom, h: here
\centering
\includegraphics[width=1.0\textwidth]{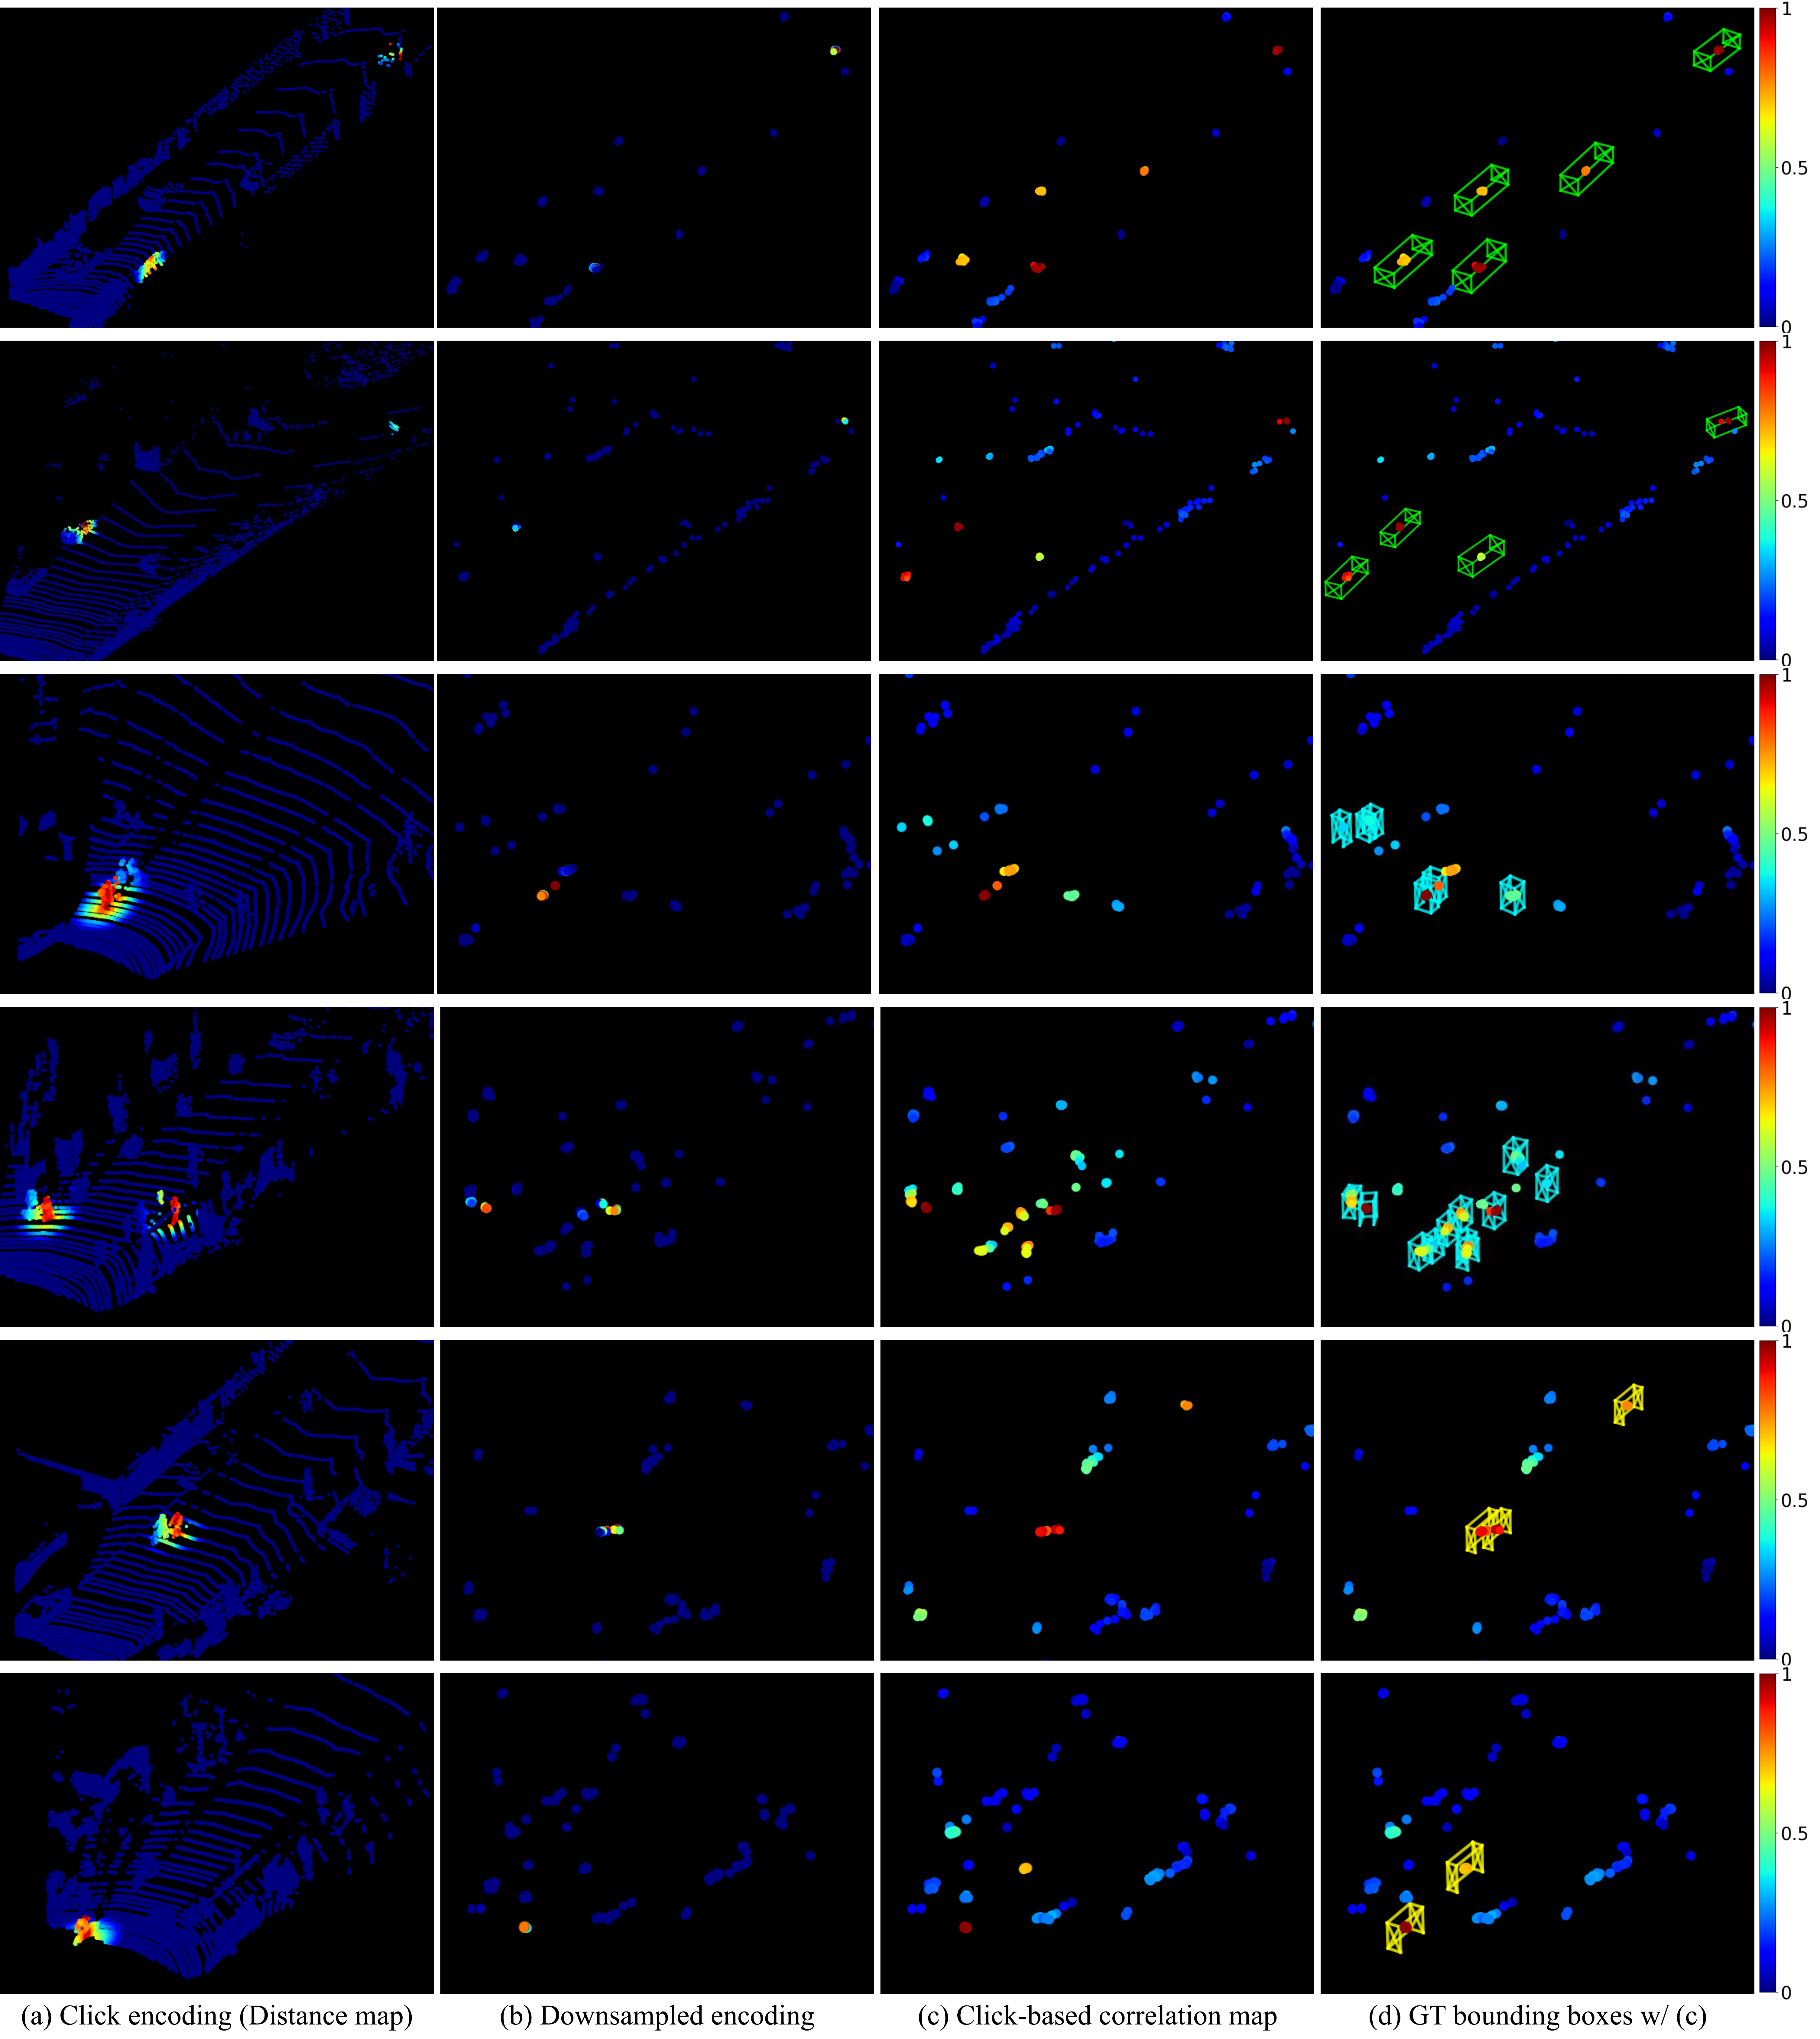}
\caption{
    More examples of correlation map generation from positive clicks using spatial click propagation (SCP) module (visualized in the scale of [0,1]).
    (Column 1) A class-wise click encoding $U$ on target objects with respect to $N$ input points.
    (Column 2) A class-wise click encoding $U'$ for $N'$ downsampled points (after point reduction from $N$ to $N'$ with downsampling layers).
    (Column 3) A class-wise correlation map $S$ generated by the SCP and
    (Column 4) visualization overlaid with the ground-truth 3D bounding boxes.
    Note that points of the same class with the click are highlighted in the output correlation map.
}

\label{supplefig:scp_pos}
\end{figure*}
