# Supplementary material for: iDet3D: Towards Efficient Interactive Object Detection for LiDAR Point Clouds
Source: arXiv:2312.15449 source file (2023-12-24)
Supplement: Supplementary file 3 [file 0_overview.tex]

\section{Overview}

This supplementary material provides further details
of our iDet3D, including the specific network architecture, more qualitative results.
In addition, we provide a \emph{demo video}
of iDet3D in comparison with the existing annotation tools.
