# Supplementary material for: iDet3D: Towards Efficient Interactive Object Detection for LiDAR Point Clouds
Source: arXiv:2312.15449 source file (2023-12-24)
Supplement: Supplementary file 4 [file 3_qualitatives.tex]

\section{Additional qualitative results}

We provide additional qualitative results produced by our iDet3D.
The extra samples are visualized in Fig.~\ref{supplefig:kitti} and Fig.~\ref{supplefig:nuscenes} on KITTI \emph{val} set and nuScenes validation split, respectively.

\begin{figure*}[t] %%% t: top, b: bottom, h: here
\centering
\includegraphics[width=1.0\textwidth]{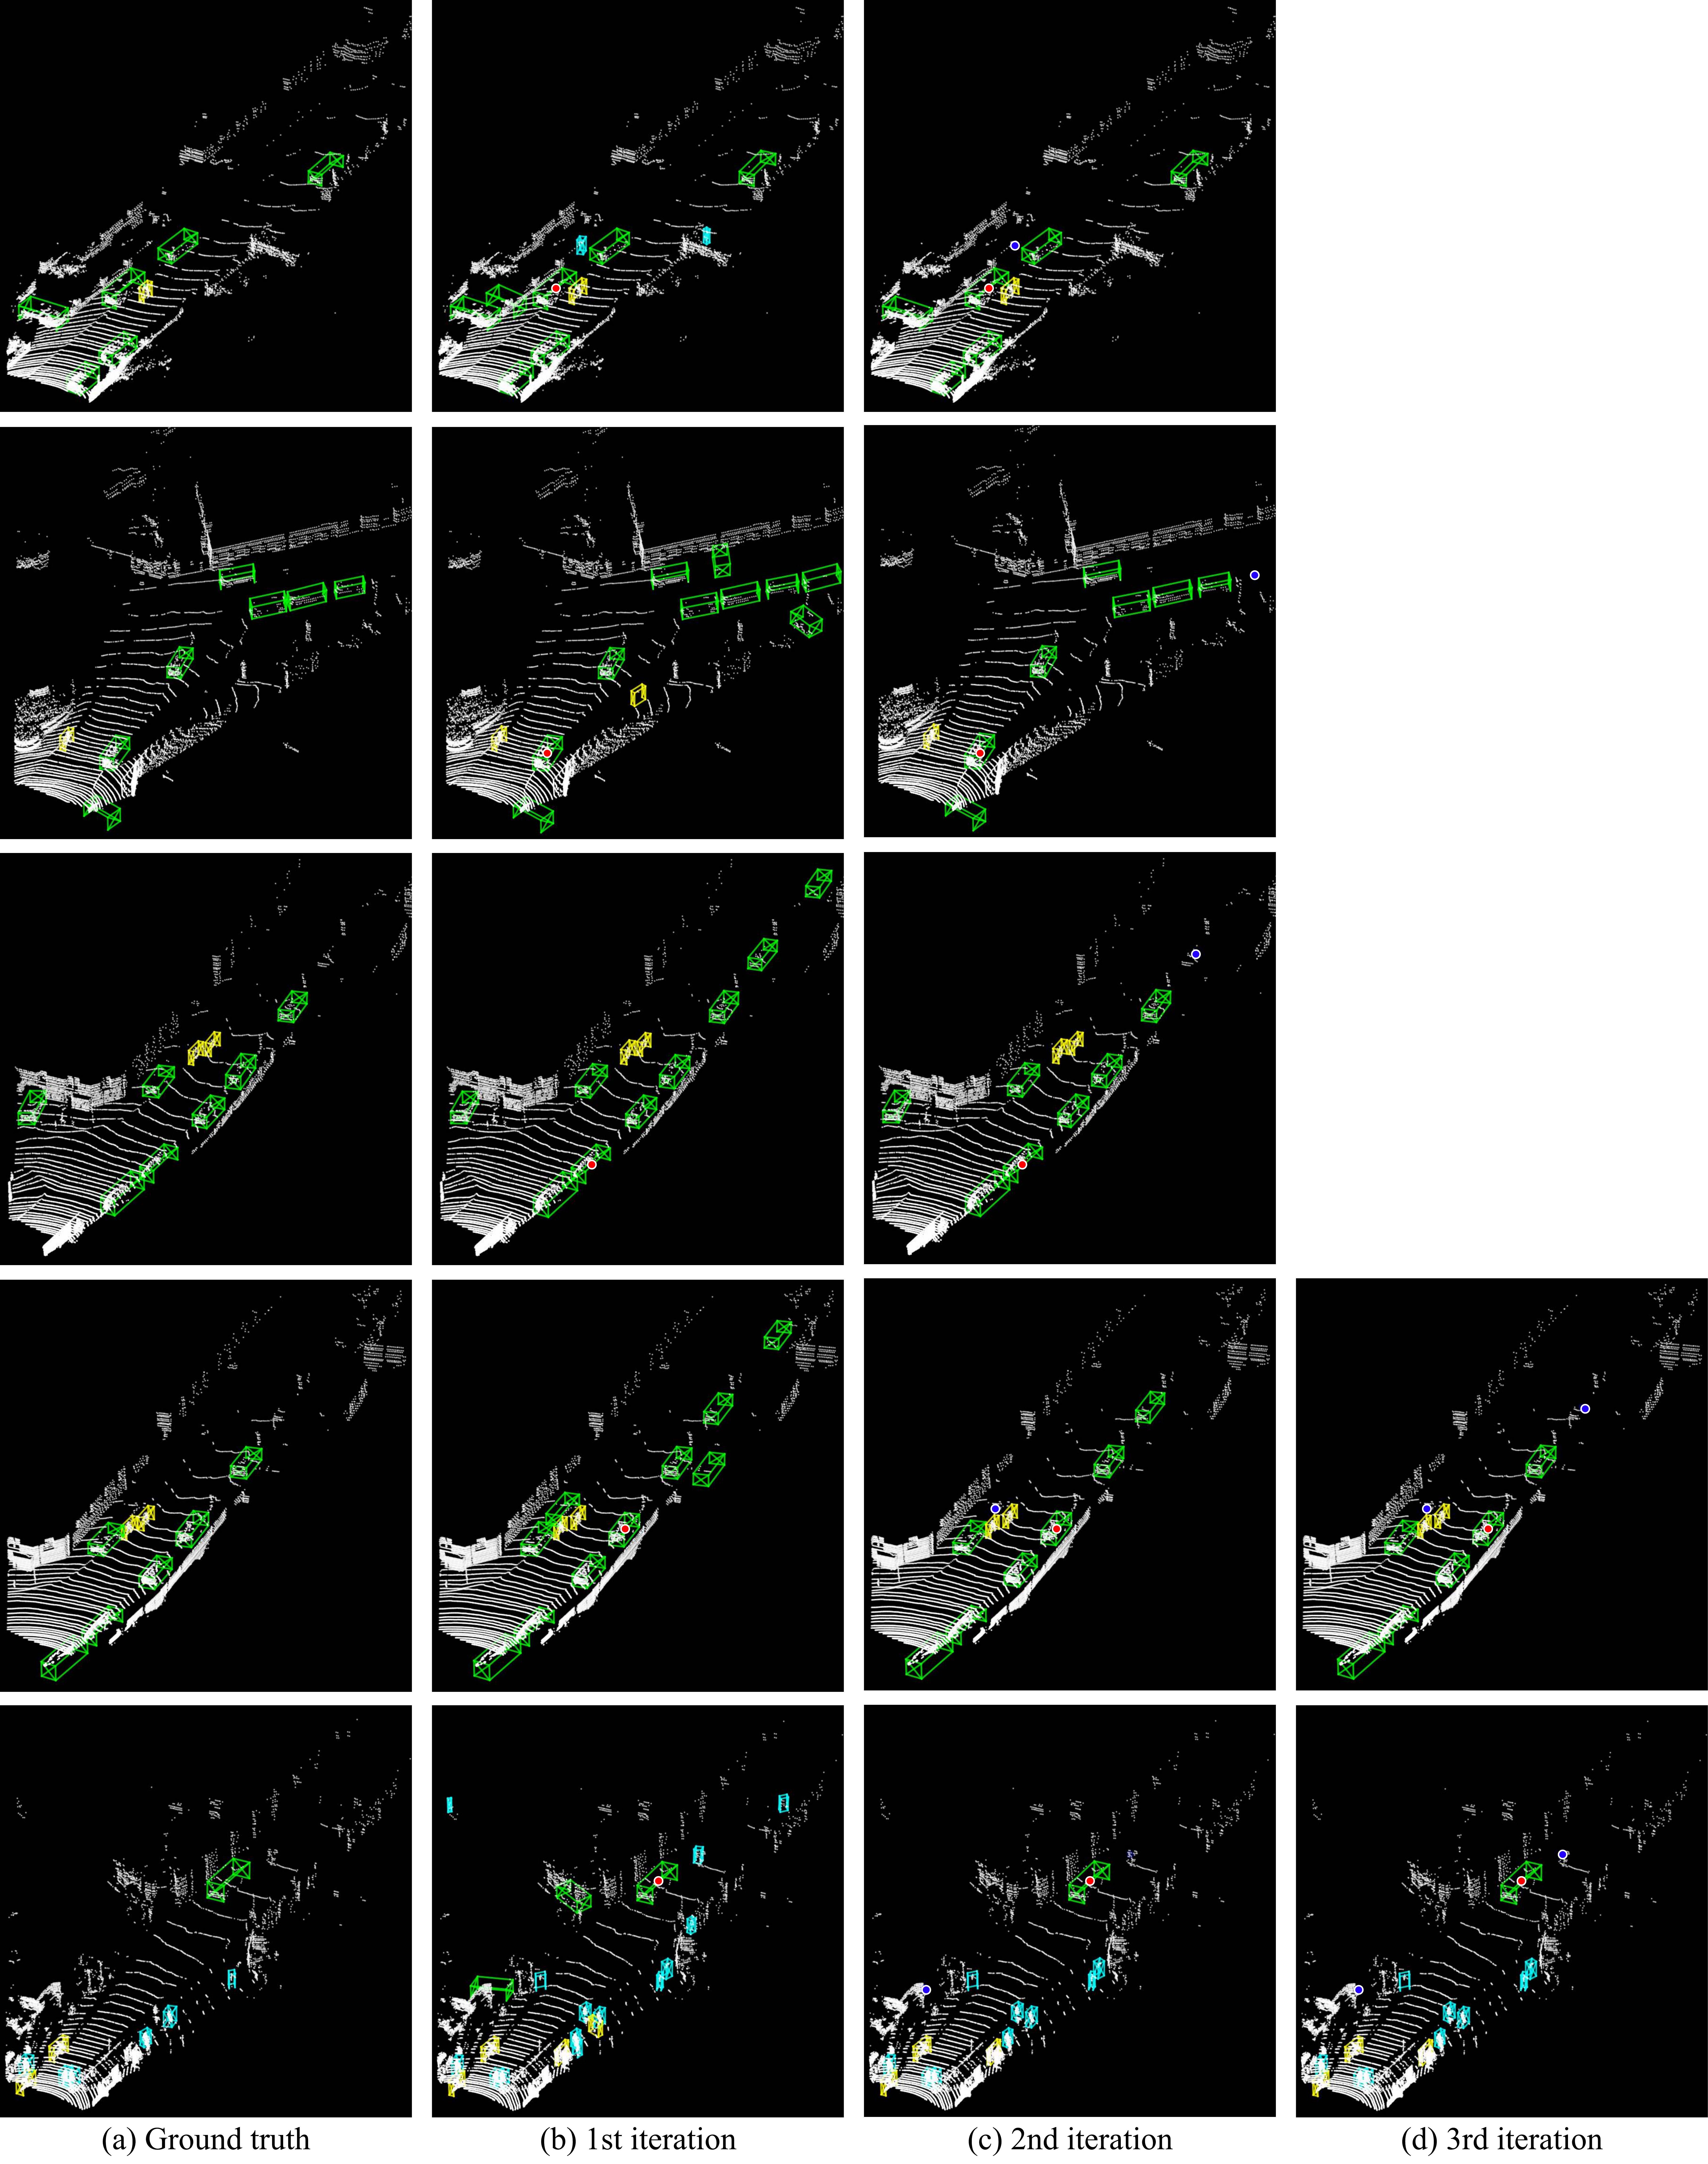}
% \vspace{-1\baselineskip}
\caption{
    Qualitative results of iDet3D on the KITTI \emph{val} set.
    \textcolor{green}{Green} boxes for Car, \textcolor{cyan}{cyan} for Pedestrian, and \textcolor{yellow}{yellow} for Cyclist with positive clicks (\textcolor{red}{red}) and negative clicks (\textcolor{blue}{blue}).
    Our iDet3D successfully detects multiple objects of different categories within two or three iterations.
}
\label{supplefig:kitti}
\end{figure*}

\begin{figure*}[t] %%% t: top, b: bottom, h: here
\centering
\includegraphics[width=1.0\textwidth]{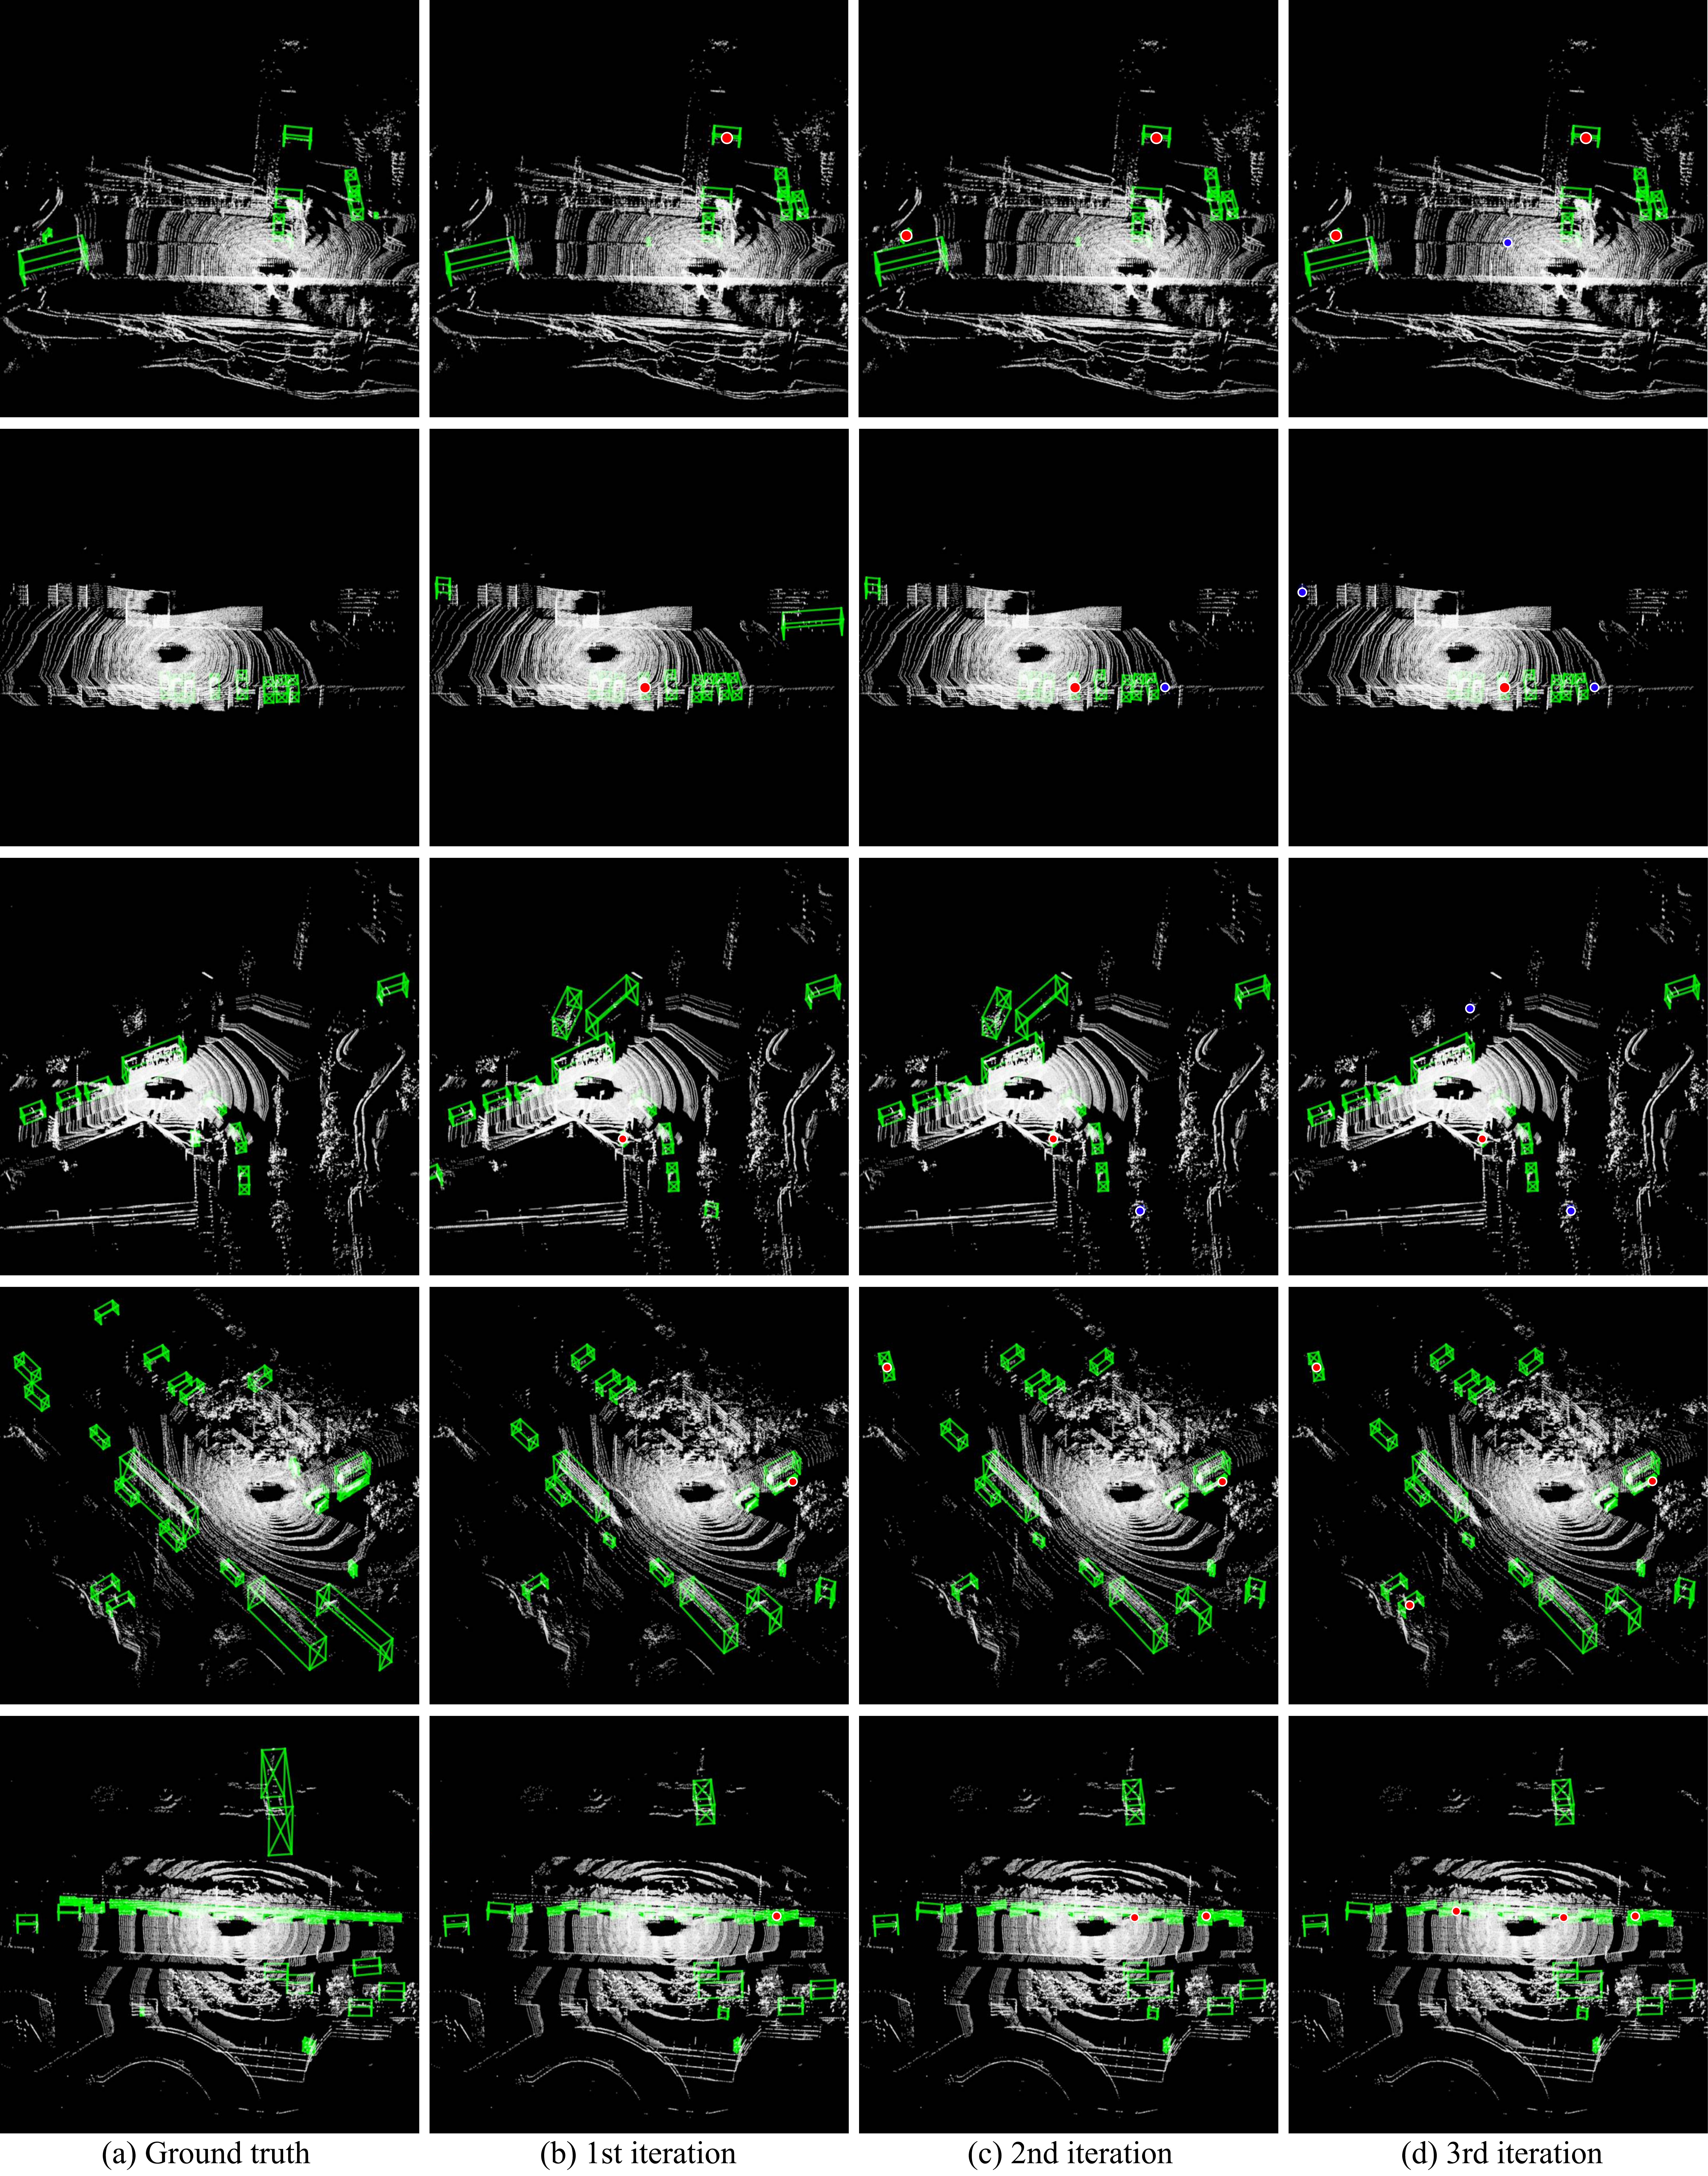}
% \vspace{-1\baselineskip}
\caption{
    Qualitative results of iDet3D on the nuScenes validation set.
    The 3D bounding boxes are colored with \textcolor{green}{green},
    and the user clicks are represented as \textcolor{red}{red} circles.
}
\label{supplefig:nuscenes}
\end{figure*}
